# Supplementary material for: Coupled networks and networks with bimodal frequency distributions are equivalent
Source: arXiv:1602.08368 source file (2016-03-03)
Supplement: Supplementary file 1 [file Pietras_etal_TwoNetworks_Supplement.pdf]

# Supplementary material – coupled networks and networks with bimodal frequency distributions are equivalent


Bastian Pietras,[1,*] Nicolás Deschle,[1,†] and Andreas Daffertshofer[1,‡]

[1] *MOVE Research Institute Amsterdam & Institute for Brain and Behavior Amsterdam, Faculty of Behavioural and Movement Sciences, Vrije Universiteit Amsterdam, van der Boechorststraat 9, Amsterdam 1081 BT, The Netherlands*



(Dated: March 3, 2016)


## BIFURCATION SCHEME FOR TWO COUPLED NETWORKS

We give a comprehensive overview of the bifurcation scheme of system (4) that read

$$\begin{aligned} \dot{q} &= q\left[1 - \Delta - q + \kappa(1-q)\cos\psi\right] \\ \dot{\psi} &= \omega_0 - \kappa(1+q)\sin\psi\ . \end{aligned} \tag{4}$$

Recall that $\Delta, \omega_0$, and $\kappa$ are the (scaled) parameters denoting the distribution widths, the distance between the peaks of the distribution functions, and the ratio of external to internal coupling, respectively. Since $q = \rho^2$ denotes the squared (local) order parameter of each subpopulation, for the solutions-of-interest we have $0 \leq q \leq 1$ and all the parameters being non-negative. We also note that for $\kappa = 0$, the external coupling $K_{\text{ext}}$ vanishes, therefore leaving two separate, non-interacting networks; see Fig. 1.

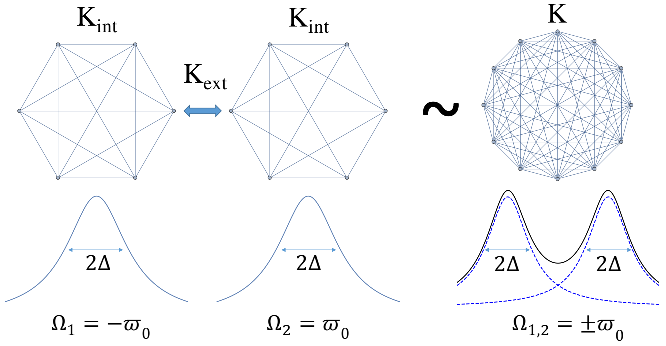


FIG. 1. Two all-to-all coupled networks (left) with unimodal frequency distributions each; a single all-to-all coupled network (right) with a symmetric bimodal frequency distribution function; cf. main text Eqs.(1&3) where details are provided.

In line with the main text, the red plane in Fig. 2 displays the supercritical Hopf bifurcation while the orange cone represents the transcritical bifurcation. Between the green curves (exact formulas in the main text) we find the saddle-node plane, which denotes the parameter values, for which a pair of a stable fixed point and a saddle point emerges as a neutral fixed point.

Along the saddle-node plane, however, we have to distinguish two cases of this bifurcation. For all points on the plane with $\Delta$ bigger than some critical value $\Delta_c$, the neutral fixed point emerges away from the stable limit cycle (for $\Delta \leq 1$), or away from the stable incoherent solution ($\Delta \geq 1$). For $\Delta \leq \Delta_c < 1$ the creation of that fixed point takes place directly on the limit cycle, where $\Delta_c$ denotes the value for the co-dimension 2 bifurcation points (blue) on the green plane in Fig. 2 — for $\kappa = 1$ this critical parameter is $\Delta = \Delta_c \approx 0.7384$. In particular, the emergent fixed point is about to split into a pair of a stable fixed point and a saddle point, therefore it destroys the limit cycle by forcing the period to infinity. This is a saddle-node infinite-period bifurcation (SNIPER). The (blue) critical curve $\Delta_c = \Delta_c(\omega_0, \kappa)$, which separates the two types of saddle-node bifurcations, consists of Bogdanov-Takens points, i.e. bifurcation points of co-dimension 2.

Furthermore, numerics reveals a plane connecting the (blue) Bogdanov-Takens curve with the (red) curve $\{\Delta = 1, \kappa = \omega_0 \,|\, \kappa, \omega_0 \geq 0\}$. The latter curve comprises the parameter values for which the saddle point (emerging from the saddle-node bifurcation) collapses with the stable incoherent solution, which then becomes unstable.

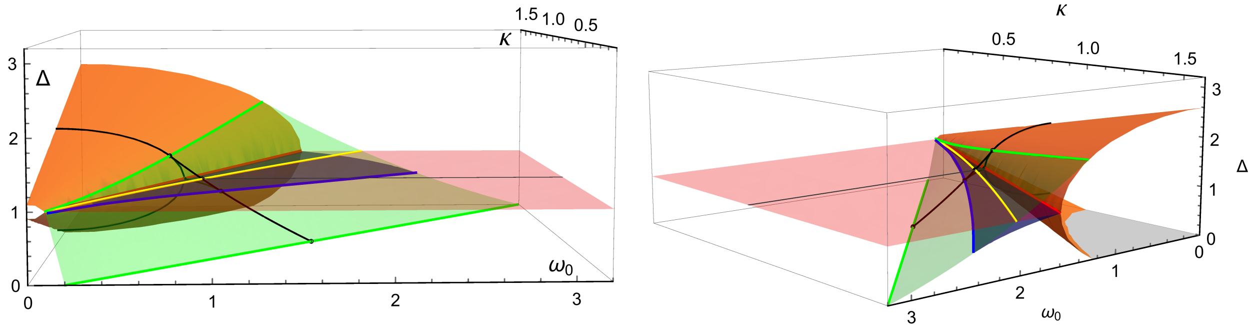


FIG. 2. Bifurcation boundaries (front and back view). Red plane: Hopf, orange cone: transcritical, green plane (within green lines): saddle node, blue: homoclinic bifurcation. Blue line: Bogdanov-Takens curve, yellow: intersection of Hopf and SN, black lines: cross-section at $\kappa = 0.8$, see also Fig. 3.

Along the blue plane in Fig. 2, a homoclinic bifurcation takes place. Here, the saddle point approaches the limit cycle, which is therefore destroyed in the end. Fig. 3 displays the cross-section at $\kappa = 0.8$ of the three-dimensional bifurcation boundaries, and elucidates the generic dynamical behavior within the corresponding parameter regions. Note that this cross-section is representative for all $\kappa > 0$ as has been proven in the main text. Unfortunately, analytical formulas for the homoclinic and Bogdanov-Takens bifurcations are still missing both in the bimodal case as well as in the subpopulation approach, so that we here rely on the numerics.

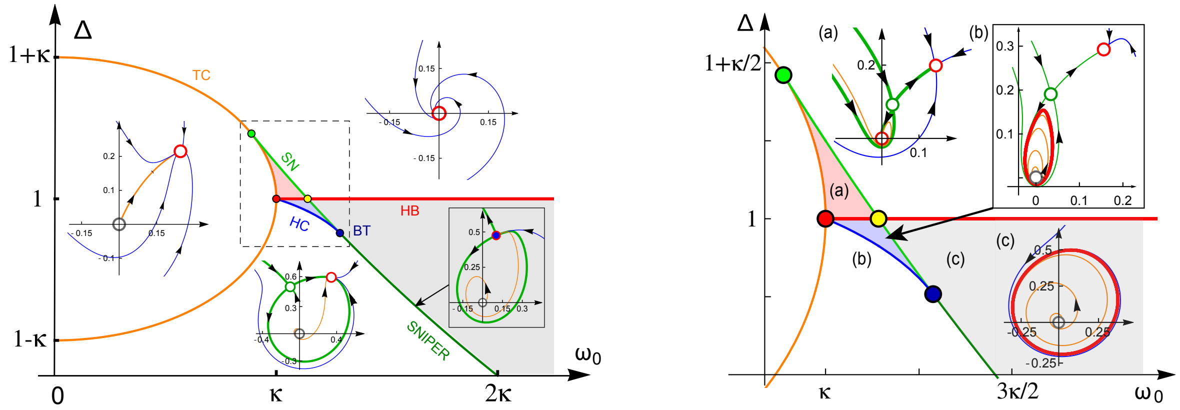


FIG. 3. Bifurcation boundaries (left) and bistability region(dashed/right): cross-section of Fig. 2 at $\kappa < 1$. Red: Hopf, orange: transcritical, green: saddle node, blue: homoclinic, blue point: Bogdanov-Takens bifurcation. Insets: $(q, \psi)$-phase portraits (in polar coordinates) in their specific parameter regions, red circle: stable, gray: unstable fixed point, green: saddle point. The right figure is a detailed view of the dashed box in the left figure.

## INFLUENCE OF TIME DELAY ON THE EFFECTIVE COUPLING STRENGTHS

An alternative case for deriving the main text's Eq. (4) is to introduce delays. For this we consider two subpopulations of oscillators that follow a unimodal frequency distribution with distinct peaks as in the left part of Fig. 1. We assume again all-to-all coupling, yet this time with the same coupling strength $K = K_{\rm int} = K_{\rm ext}$ within as well as across subpopulation boundaries. By contrast, however, we introduce population-specific time delays $\tau_{\sigma,\sigma'}$, such that the dynamics of the $k$-th oscillator of population $\sigma$ is governed by

$$\dot{\theta}_{\sigma,k}(t) = \omega_{\sigma,k} + \frac{K}{N}\sum_{\sigma'=1}^{2}\sum_{j=1}^{N}\sin\left(\theta_{\sigma',j}\left(t-\tau_{\sigma',\sigma}\right) - \theta_{\sigma,k}(t)\right) \ ,$$

where $k = 1, \ldots, N$ and $\sigma = 1, 2$. For simplicity, we consider the time delay within populations to be negligible compared to that across boundaries, hence without loss of generality we have $\tau_{\sigma,\sigma'} = 0$ and $\tau_{\sigma,\sigma} = \tau > 0$. If we further

assume the time delay $\tau \ll 2\pi/\omega_0$ and also the coupling strength $K$ being sufficiently small, we can approximate $\theta_{\sigma',j}(t-\tau)$ by means of Taylor such that

$$\theta_{\sigma',j}(t-\tau) \approx \theta_{\sigma',j}(t) - \tau\,\dot{\theta}_{\sigma',j}(t) \approx \theta_{\sigma',j}(t) - \tau\left[\overline{\omega}_{\sigma'} + \mathcal{O}(K)\right] \approx \theta_{\sigma',j}(t) - \alpha_{\sigma'}\ ,$$

where $\alpha_{\sigma'} = \tau\overline{\omega}_{\sigma'}$ with $\overline{\omega}_{\sigma'} = \pm\varpi_0$. Hence, we can replace the time delay by phase lag parameters, cf.[1, 2]. The population-specific phase lag parameters depend on the mean frequency of the oscillators, such that we have $\gamma := \alpha_1 = -\alpha_2$. Consequently, the governing equations read

$$\dot{\theta}_{1,k} = \omega_{1,k} + \frac{K}{N}\sum_{j=1}^{N}\sin(\theta_{1,j}-\theta_{1,k}) + \frac{K}{N}\sum_{j=1}^{N}\sin(\theta_{2,j}-\theta_{1,k}-\gamma)$$

$$\dot{\theta}_{2,k} = \omega_{2,k} + \frac{K}{N}\sum_{j=1}^{N}\sin(\theta_{2,j}-\theta_{2,k}) + \frac{K}{N}\sum_{j=1}^{N}\sin(\theta_{1,j}-\theta_{2,k}+\gamma)\ .$$

Now, we use again the Ott-Antonsen theory and perform the same steps for this system as we have done in the main text. We end up with the dynamics for the local order parameters

$$\dot{z}_\sigma = -(\Lambda_\sigma - i\Omega_\sigma)z_\sigma + \frac{K}{2}z_\sigma\left(1-|z_\sigma|^2\right) + \frac{K}{2}\mathrm{e}^{-i\gamma}\left(z_{\sigma'} - z_\sigma^2 z_{\sigma'}^* \mathrm{e}^{2i\gamma}\right)\ ,$$

where we have let the oscillators' frequencies follow symmetric Lorentzians, $g_\sigma(\omega) = (\Lambda_\sigma/\pi)/(((\omega-\Omega_\sigma)^2 + \Lambda_\sigma^2)^2)$, with $\Lambda_1 = \Lambda_2 =: \Lambda$ and $\Omega_1 = \varpi_0 = -\Omega_2$. As in the main text, we further introduce polar coordinates for the local order parameters, $z_\sigma = \rho_\sigma \mathrm{e}^{i\phi_\sigma}$. For symmetry reasons we set $\rho := \rho_1 = \rho_2$, and let $\Psi$ denote the difference of the mean phases. Then, we scale according to $\tilde{t} = \frac{K}{2}t, \Delta = \frac{4\Lambda}{K}, \omega_0 = \frac{4\varpi_0}{K}$ and write $q = \rho^2$. Hence, we arrive at

$$\dot{q} = q\left[1 - \Delta - q + (1-q)\cos(\psi+\gamma)\right]$$

$$\dot{\psi} = \omega_0 - (1+q)\sin(\psi+\gamma)\ ,$$

where the dot-notation refers to the derivative with respect to $\tilde{t}$. In particular, this is exactly the same system (4) as in the main text for $\kappa = 1$, and as Eqs.(25&26) in Martens et al. [3]. Merely, the mean phase difference is shifted by the (constant) phase lag parameter $\gamma$. But due to the $2\pi$-periodicity of $\Psi$, this phase shift does not alter the original dynamics.

Therefore, we may conclude that population-specific time delay does not change the effective coupling strengths, as would have led to $\kappa \neq 1$ in system (4). Note, however, that our derivation was based on a restricted size of time delays. If allowing more general time delays, the phase lag approximation cannot hold anymore. As has been shown, e.g., by Yeung and Strogatz in [4], already one single network with time delay can exhibit bistability and an oscillating order parameter. Hence, we may expect that the dynamics of two coupled networks may reveal even more delicate synchronization patterns, which await to be explored.

* b.pietras@vu.nl
† n.deschle@vu.nl
‡ a.daffertshofer@vu.nl
[1] E. M. Izhikevich, Physical Review E **58**, 905 (1998).
[2] M. J. Panaggio and D. M. Abrams, Nonlinearity **28**, R67 (2015).
[3] E. A. Martens, E. Barreto, S. H. Strogatz, E. Ott, P. So, and T. M. Antonsen, Phys. Rev. E **79**, 026204 (2009).
[4] M. S. Yeung and S. H. Strogatz, Physical Review Letters **82**, 648 (1999).
